# Supplementary material for: Quantifying non-stabilizerness through entanglement spectrum flatness
Source: arXiv:2304.01175 source file (2024-05-08)
Supplement: Supplementary file 1 [file suppmat.pdf]

# Supplemental Material

Emanuele Tirrito,[1,2] Poetri Sonya Tarabunga,[1,2,3] Gugliemo Lami,[2] Titas Chanda,[1,2] Lorenzo Leone,[4] Salvatore F.E. Oliviero,[4] Marcello Dalmonte,[1,2] Mario Collura,[2,3] and Alioscia Hamma[5,6]
[1]*The Abdus Salam International Centre for Theoretical Physics (ICTP), Strada Costiera 11, 34151 Trieste, Italy*
[2]*SISSA, Via Bonomea 265, 34136 Trieste, Italy*
[3]*INFN, Sezione di Trieste, Via Valerio 2, 34127 Trieste, Italy*
[4]*Physics Department, University of Massachusetts Boston, 02125, USA*
[5]*Dipartimento di Fisica 'Ettore Pancini', Università degli Studi di Napoli Federico II, Via Cintia 80126, Napoli, Italy*
[6]*INFN, Sezione di Napoli, Italy*

## Proof of Theorem

Let us recall the measure of entanglement spectrum flatness for a pure state $|\psi\rangle$ in the bipartition $A \cup B$ defined in the main text

$$\mathcal{F}_A(|\psi\rangle) = \mathrm{Tr}(\rho_A^3) - \mathrm{Tr}^2(\rho_A^2) \tag{S1}$$

where $\rho_A = \mathrm{Tr}_B |\psi\rangle\langle\psi|$. In this section, we compute the average over the Clifford orbit $\Gamma|\psi\rangle$ where $\Gamma \in C_n$, i.e. $\langle \mathcal{F}_A(\Gamma|\psi\rangle)\rangle_{C_n}$. Note that we can write

$$\langle \mathcal{F}_A(\Gamma|\psi\rangle)\rangle_{C_n} = \langle \mathrm{Tr}(\rho_{\Gamma,A}^3)\rangle_{C_n} - \langle \mathrm{Tr}^2(\rho_{\Gamma,A}^2)\rangle_{C_n} \tag{S2}$$

where $\rho_{\Gamma,A} = \mathrm{Tr}_B(\Gamma|\psi\rangle\langle\psi|\Gamma^\dagger)$. We can now use the swap trick, i.e. $\mathrm{Tr}(O^3) = \mathrm{Tr}(T_{(123)}O^{\otimes 3})$ and $\mathrm{Tr}^2(O^2) = \mathrm{Tr}(T_{(12)(34)}O^{\otimes 4})$ to linearize the above averages over multiple copies of $|\psi\rangle$

$$\begin{aligned}\langle \mathcal{F}_A(\Gamma|\psi\rangle)\rangle_{C_n} &= \mathrm{Tr}(T^A_{(123)}\,\langle(\Gamma|\psi\rangle\langle\psi|\Gamma^\dagger)^{\otimes 3}\rangle_{C_n}) \\ &- \mathrm{Tr}(T^A_{(12)(34)}\,\langle(\Gamma|\psi\rangle\langle\psi|\Gamma^\dagger)^{\otimes 4}\rangle_{C_n})\end{aligned} \tag{S3}$$

where $T^A_{(123)}$ and $T^A_{(12)(34)}$ are permutations acting non-identically on the subsystem $A$ only. For the first average in the r.h.s. of Eq. (S3), we use the fact that the Clifford group is a 3-design [S1, S2] and thus

$$\langle(\Gamma|\psi\rangle\langle\psi|\Gamma^\dagger)^{\otimes 3}\rangle_{C_n} = \frac{\Pi^{(3)}_{sym}}{\mathrm{Tr}(\Pi^{(3)}_{sym})} \tag{S4}$$

where $\Pi^{(3)}_{sym} = \sum_{\pi_3\in S_3} T_{\pi_3}/3!$ is the symmetric projector, $S_3$ is the symmetric group acting on 3 copies of the Hilbert space of $n$ qubits and $T_{\pi_3}$ are unitary representations of permutations $\pi_3 \in S_3$. Therefore, the first term in Eq. (S3) can be computed as

$$\frac{1}{\mathrm{Tr}\,\Pi^{(3)}_{sym}}\mathrm{Tr}(T^A_{(123)}\Pi^{(3)}_{sym}) = \frac{\sum_{\pi\in S_3}}{\mathrm{Tr}\,\Pi^{(3)}_{sym}}\mathrm{Tr}_A(T^A_{(123)}T^A_\pi)\,\mathrm{Tr}_B(T^B_\pi) \tag{S5}$$

where we used the fact that any permutation operator $T_\pi$ for $\pi \in S_3$ obey $T_\pi = T^A_\pi \otimes T^B_\pi$. For the second average of the r.h.s. of Eq. (S3), we use the technical results presented in [S3, S4] that shows

$$\langle(\Gamma|\psi\rangle\langle\psi|\Gamma^\dagger)^{\otimes 4}\rangle_{C_n} = \alpha Q\Pi^{(4)}_{sym} + \beta\Pi^{(4)}_{sym} \tag{S6}$$

where $Q = d^{-2}\sum_{P\in\mathcal{P}_n} P^{\otimes 4}$ and $\Pi^{(4)}_{sym}$ is the symmetric projector on $S_4$, defined as $\Pi^{(4)}_{sym} \equiv \sum_{\pi_4\in S_4} T_{\pi_4}/4!$. Then we defined

$$\begin{aligned}\alpha &:= \frac{\|\Xi_\psi\|_2^2}{(d+1)(d+2)/6} - \beta \\ \beta &:= \frac{1-\|\Xi_\psi\|_2^2}{(d^2-1)(d+2)(d+4)/24}\end{aligned} \tag{S7}$$

Therefore, the second term in Eq. (S3) can be computed as

$$\begin{aligned}\langle \mathrm{Tr}^2(\rho^2_{\Gamma,A})\rangle_{C_n} &= \mathrm{Tr}[T^A_{(12)(34)}(\alpha Q + \beta I)\Pi^{(4)}_{sym}] \\ &= \sum_{\pi\in S_4}[\alpha\,\mathrm{Tr}_A(T^A_\pi T^A_{(12)(34)}Q^A)\,\mathrm{Tr}_B(T^B_\pi Q^B) \\ &+ \beta\,\mathrm{Tr}_A(T^A_\pi T^A_{(12)(34)})\,\mathrm{Tr}_B(T^B_\pi)]\end{aligned} \tag{S8}$$

where we used the fact that $Q = Q_A \otimes Q_B$ and $Q_X = d_X^{-2}\sum_{P\in\mathcal{P}_X} P_X^{\otimes 4}$ for $X = A, B$. Notice that $\mathrm{Tr}(QT_\pi)$ are computed in [S3] and tabulated in [S5]. After a straightforward algebra, recalling that $M_{lin}(|\psi\rangle) = 1 - d\|\Xi_\psi\|_2^2$, one finds:

$$\begin{aligned}\langle \mathcal{F}_A(\mathrm{Tr}_B(\Gamma|\psi\rangle\langle\psi|\Gamma^\dagger))\rangle_{C_n} &= \frac{(d^2-d_A^2)(d_A^2-1)}{(d^2-1)(d+2)d_A^2}M_{lin}(|\psi\rangle) \\ &\equiv c(d,d_A)M_{lin}(|\psi\rangle)\end{aligned} \tag{S9}$$

which concludes the proof. □

## Proof of Proposition

Let us recall the definition of stabilizer fidelity

$$\mathcal{S}_{\max}(\psi) = \max_{\sigma\in\mathrm{STAB}} |\langle\sigma|\psi\rangle|^2 \tag{S10}$$

and let us first prove the following lemma.

**Lemma:** *Given a pure state $|\psi\rangle$ and a bipartition $A|B$, then we have that the flatness $\mathcal{F}_A$ is upper bounded by*

$$\mathcal{F}_A(\psi) \le 7\sqrt{1-\mathcal{S}_{\max}(\psi)} \tag{S11}$$

*Proof.—* Notice that for every stabilizer state $\sigma$ we have $\mathcal{F}_A(\sigma) = 0$. Then, we have the following chain of inequal-

ities

$$\begin{aligned}
&\mathcal{F}_A(\psi) = \mathcal{F}_A(\psi) - \mathcal{F}_A(\sigma)\\
=&\ \mathrm{Tr}[T^{(A)}_{123}(\psi^{\otimes 3} - \sigma^{\otimes 3})] - \mathrm{Tr}[T^{(A)}_{(12)(34)}(\psi^{\otimes 4} - \sigma^{\otimes 4})]\\
\leq&\ |\,\mathrm{Tr}[T^{(A)}_{123}(\psi^{\otimes 3} - \sigma^{\otimes 3})]| + |\,\mathrm{Tr}[T^{(A)}_{(12)(34)}(\psi^{\otimes 4} - \sigma^{\otimes 4})]|\\
\leq&\ \|T^{A}_{(123)}\|_\infty \|\psi^{\otimes 3} - \sigma^{\otimes 3}\|_1 + \|T^{A}_{(12)(34)}\|_\infty \|\psi^{\otimes 4} - \sigma^{\otimes 4}\|_1\\
=&\ 7\|\psi - \sigma\|_1 = 7\sqrt{1 - |\langle\sigma|\psi\rangle|^2} \qquad \text{(S12)}
\end{aligned}$$

in the second line, we used the definition of Flatness used in the paper. In the third line, we used triangle inequality. In the fourth line we used the bound of Schatten $p$-norms, namely $|\,\mathrm{Tr}(AB)| \leq \|A\|_p \|A\|_q$ for $p^{-1} + q^{-1} = 1$ and chosen $p = \infty$ and $q = 1$. In the last line, we made use of the following inequality multiple times

$$\begin{aligned}
\|\psi^{\otimes 4} - \sigma^{\otimes 4}\| &= \|\psi^{\otimes 4} - \psi \otimes \sigma^{\otimes 3} + \psi \otimes \sigma^{\otimes 3} - \sigma^{\otimes 4}\|\\
&\leq \|\psi\|\|\psi^{\otimes 3} - \sigma^{\otimes 3}\| + \|\psi - \sigma\|\|\sigma^{\otimes 3}\|\\
&= \|\psi^{\otimes 3} - \sigma^{\otimes 3}\| + \|\psi - \sigma\|\\
&\leq 4\|\psi - \sigma\| \qquad \text{(S13)}
\end{aligned}$$

Then choosing in Eq. (S13) $\min_{\sigma\in\mathrm{STAB}}$, one obtain Eq. (S11). □

The proposition in the main text is now a corollary of the above lemma. Indeed given the threshold $\epsilon$ for the algorithm in Fig. 1 panel (c), then if $\mathcal{S}_{\max} > 1 - \epsilon^2/7$ then $\mathcal{F}_A(\psi) < \epsilon$ and thus $\mathcal{P}_{\mathrm{Suc}}(\epsilon) = 0$. □

### *Stabilizer fidelity and stabilizer entropy*

Let us now discuss the implications of the above result and the relationship between the stabilizer fidelity and the stabilizer entropy. The stabilizer fidelity and the stabilizer entropy are interconnected through the inequality [S6]$M_{lin} \leq 1 - \mathcal{S}^4_{\max}(\psi)$, which presents an intriguing relationship. However, for the purpose of the failure of the algorithm and the proposition presented in the main text earlier, this relationship does not provide significant assistance. We can just infer that if $\mathcal{S}_{\max} > 1 - \epsilon^2/7$, then $M_{lin} \lesssim \frac{4}{7}\epsilon^2$.

Strong numerical evidence [S6] suggested that for $M_{\mathrm{lin}}$, the following inequality holds:

$$1 - \mathcal{S}^a_{\max} \leq M_{lin}, \qquad \text{(S14)}$$

for $a \simeq 1.7$. This finding provides a useful lower bound for the linear stabilizer entropy. Therefore, these results suggest a direct connection between the failures of the protocol and the linear stabilizer entropy, as numerically shown in the plot of Fig. 1 panel (c). Assuming (S14), then we would have $\mathcal{F}_A(\psi) \leq 7\sqrt{1 - (1 - M_{\mathrm{lin}})^{1/a}}$, thus providing a direct relationship between the failure of the witness algorithm and the linear stabilizer entropy.

### Clifford circuit

Let us start by describing the architecture of a random Clifford circuit, both with and without noise. We consider a system of $n$ qubits with a Hilbert space $\mathcal{H} = \bigotimes_{j=1}^n \mathbb{C}^2$. The group $P_n$ comprises all $n$-qubit Pauli strings with phases $\pm 1$ and $\pm i$. The Clifford group $C(d)$ consists of unitary operators that transform Pauli strings into Pauli strings. In other words, for any $\Gamma \in C(d)$, we have $\Gamma P \Gamma^\dagger \in P_n$ for all $P \in P_n$. The Clifford group can be generated by three gates: the Hadamard gate, the phase gate $e^{i\pi/2}$ (S gate), and the CNOT gate. Since the phase and Hadamard gates can construct all Pauli matrices, each Pauli gate is also an element of the Clifford group.

In the case of a random Clifford circuit without noise, the state $|\psi_0\rangle$ evolves under a random Clifford circuit of depth $N_{\mathrm{Layers}}$ denoted as $U_{\mathrm{Cl}} = \prod_k^{N_{\mathrm{Layers}}} U_k$. Here, $U_k$ contains $n-1$ Clifford gates (Hadamard, S gate, and CNOT) between nearest neighbors.

Additionally, the Clifford unitaries exhibit residual noise due to the fine-tuning involved in constructing these circuits. To account for this, we consider a simple error model where each two-qubit Clifford gate $U_k$ is affected by unitary noise, as described in Eq. (6). Specifically, only the CNOT gate is affected by the error. Utilizing Eq. (6), the modified CNOT gate $\tilde{C}_{\mathrm{NOT}}$ can be expressed as:

$$\begin{aligned}
\tilde{C}_{\mathrm{NOT}} &= e^{-i\sum_\alpha \epsilon_\alpha P^\alpha} \begin{pmatrix} 1 & 0 \\ 0 & X \end{pmatrix} e^{i\sum_\alpha \epsilon_\alpha P^\alpha} \qquad \text{(S15)}\\
&= \begin{pmatrix} 1 & 0 \\ 0 & e^{-i\sum_\alpha \epsilon_\alpha P^\alpha} X e^{i\sum_\alpha \epsilon_\alpha P^\alpha} \end{pmatrix}.
\end{aligned}$$

In the presence of noise, the state $|\psi_0\rangle$ undergoes evolution under a random circuit of depth $N_{\mathrm{Layers}}$, denoted as $\tilde{U} = \prod_k^{N_{\mathrm{Layers}}} \tilde{U}_k$. Here, $\tilde{U}k$ comprises $n-1$ Clifford gates randomly chosen from the set of the Hadamard gate, S gate, and $\tilde{C}_{\mathrm{NOT}}$.


[S1] H. Zhu, Phys. Rev. A **96**, 062336 (2017).

[S2] H. Zhu, R. Kueng, M. Grassl, and D. Gross, The Clifford group fails gracefully to be a unitary 4-design (2016), arXiv:1609.08172.

[S3] L. Leone, S. F. E. Oliviero, Y. Zhou, and A. Hamma, Quantum **5**, 453 (2021).

[S4] S. F. Oliviero, L. Leone, and A. Hamma, Physics Letters A **418**, 127721 (2021).

[S5] L. Leone, Mathematica script for clifford group and beyond. `https://github.com/lorenzoleone/Clifford-group-and-beyond` (2023).

[S6] T. Haug and L. Piroli, Stabilizer entropies and nonstabilizerness monotones (2023), arXiv:2303.10152.
